# Supplementary material for: Efficient Selection Between Hierarchical Cognitive Models: Cross-validation With Variational Bayes
Source: arXiv:2102.06814 source file (2021-10-08)
Supplement: Supplementary file 1 [file Appendix.tex]

\begin{center}
		\section*{Appendix}
	\end{center}
	
	\subsection*{Derivation the gradients for LBA models}
	$\joint = \like\prior = p(\by|\balph)p(\balph|\bmu,\bSigalph)p(\bmu)p(\bSigalph|a_1,\dots,a_D)\prod\limits_{d=1}^D p(a_d)$.\\
	In order to approximate $\post$ using the variational approximation methods described above, we need to obtain from the model the gradient $\nabla_{\btheta}\logjoint$ or equivalently, $\nabla_\theta \log \like$ and $\nabla_\theta \logprior$\\
	\subsubsection*{$\boldsymbol{\nabla_{\bthetatilde} \log \like}$}
	
	It is obvious that $\nabla_{\bmualph} \loglike = \boldsymbol{0},\, \nabla_{\vech(\bCstar)} \loglike  = \boldsymbol{0}, \nabla_{\log\ba} \loglike  = \boldsymbol{0}$ (since $\like = p(\by|\balph_{1:J})$ \\
	
	$\nabla_{\balph_k} \loglike = \dfrac{\partial}{\partial \balph_k} \log p(\by_k|\balph_k)= \sum\limits_{j=1}^{n_k} \dfrac{\partial}{\partial \balph_k} \log p(y_{kj}|\balph_k) =\sum\limits_{j=1}^{n_k} \dfrac{ \dfrac{\partial}{\partial \bz_k} p(y_{kj}|\bz_k) \dfrac{\partial \bz_k}{\partial \balph_k} }{p(y_{kj}|\bz_k)} $\\
	
	%$\dfrac{\partial}{\partial \balph_k} \log p(y_{kj}|\balph_k) =$\\
	$\dfrac{\partial}{\partial \bz_k} p(y_{kj}|\bz_k) = \dfrac{\partial}{\partial \bz_k}f_c(t)(1 - F_{\overline{c}}(t)) + \dfrac{\partial}{\partial \bz_k}(1 - F_{\overline{c}}(t))f_c(t)$\\
	
	\vspace*{0.5cm}
	\hspace*{-0.5cm}Derivatives of $f_c(t)$ with respect to $\bz$\\
	
	$\dfrac{\partial}{\partial b}f_c(t) = \dfrac{1}{A}\bigg[  -v^c\xone + s\xtwo + v^c\zone - s\ztwo \bigg]\dfrac{\partial \wone}{\partial b}$\\
	
	$\dfrac{\partial}{\partial A}f_c(t) = -\dfrac{1}{A}\bigg[  f_c(t) - v^c\xone + s\xtwo\bigg]\dfrac{\partial \wone}{\partial A}$\\
	
	$\dfrac{\partial}{\partial v^c}f_c(t) = \dfrac{1}{A}\bigg[  - \xzero +\zzero\bigg] + \dfrac{1}{A}\bigg[  - v^c\xone+s\xtwo+v^c\zone-s\ztwo\bigg]\dfrac{\partial \wone}{\partial v^c}$\\
	
	$\dfrac{\partial}{\partial \tau}f_c(t) = \dfrac{1}{A}\bigg[   - v^c\xone +s\xtwo \bigg]\left( \dfrac{\partial \wone}{\partial \tau} -\dfrac{\partial \wtwo}{\partial \tau} \right) + \dfrac{1}{A}\bigg[    v^c\zone-s\ztwo\bigg]\dfrac{\partial \wone}{\partial \tau}$\\
	
	\vspace*{0.5cm}
	\hspace*{-0.5cm}Derivatives of $F_c(t)$ with respect to $\bz$\\
	
	$\begin{array}{ll}
	
	\dfrac{\partial}{\partial b}F_c(t) &= \bigg[\dfrac{1}{A}\xzero +\uone\xone\dfrac{\partial \wone}{\partial b} \bigg]\\
	&+\dfrac{1}{\wtwo} \bigg[\xtwo-\ztwo \bigg]\dfrac{\partial \wone}{\partial b}+ \bigg[ -\dfrac{1}{A}\zzero - \utwo\zone \dfrac{\partial \wone}{\partial b} \bigg]\\
	
	\dfrac{\partial}{\partial A}F_c(t) &= \dfrac{1}{A}\bigg[-\xzero +\xone(b-A-(t-\tau)v^c)\dfrac{\partial \wtwo}{\partial A} \bigg]\\
	&+\dfrac{1}{A^2}\bigg[ (b-(t-\tau)v^c)\zzero-(b-A-(t-\tau)v^c)\xzero \bigg]\\
	&+ \dfrac{\xtwo\dfrac{\partial \wtwo}{\partial A}\wtwo - \dfrac{\partial \wtwo}{\partial A}\xone }{\wtwo^2}+\zone\dfrac{\partial \wtwo}{\partial A}\\
	
	\dfrac{\partial}{\partial v^c}F_c(t) &= -\dfrac{t-\tau}{A}\xzero+\uone\xone\dfrac{\partial \wone}{\partial v^c}\\
	&+\dfrac{t-\tau}{A}\zzero - \zone\utwo\dfrac{\partial \wone}{\partial v^c}\\
	&+\dfrac{1}{\wtwo}\left( \xtwo-\ztwo\right)\dfrac{\partial \wone}{\partial v^c}\\
	
	\dfrac{\partial}{\partial \tau}F_c(t) &=\dfrac{v^c}{\tau}\xzero+\uone\xone\left( \dfrac{\partial \wone}{\partial \tau} -\dfrac{\partial \wtwo}{\partial \tau} \right) \\
	&-\dfrac{v^c}{\tau}\zzero-\utwo\zone\dfrac{\partial \wone}{\partial \tau} \\
	&+\bigg[\xtwo\wtwo\left( \dfrac{\partial \wone}{\partial \tau} -\dfrac{\partial \wtwo}{\partial \tau} \right)-\xone\dfrac{\partial \wtwo}{\partial \tau} \bigg]/(\wtwo^2)\\
	&-\bigg[\ztwo\wtwo\dfrac{\partial \wone}{\partial \tau}-\zone\dfrac{\partial \wtwo}{\partial \tau} \bigg]/(\wtwo^2)
\end{array}$

\subsubsection*{$\boldsymbol{\nabla_{\bthetatilde} \logpriortilde}$}

$$\bthetatilde = (\balph_{1:J},\bmualph,\vech(\bCstar),\log a_{1:\Da}) $$
\begin{align*}
    \priortilde = &p(\balph_{1:J}|\bmualph,\bSigalph)\times p(\bmualph|\bmu,\bSig)\times p(\vech(\bCstar)|\log a_{1:\Da})\times p(\log a_{1:\Da})\\
    = &\prod\limits_{j=1}^J N(\balph_{j}|\bmualph,\bSigalph)\times N(\bmualph|\bmu,\bSig)\times \textrm{IW}(\bSigalph|\nu,\bPsi)\times \left|J_{\bSigalph\rightarrow \vech(\bCstar)}\right|\times\cdots \\
    &\times \prod\limits_{d=1}^D \textrm{IG}(a_d|\alpha_d,\beta_d)\times \left|J_{a_{1:\Da}\rightarrow \log a_{1:\Da}} \right|
\end{align*}
with the prior hyperparameters:\\
\begin{itemize}
    \item[-] $\bmu = \boldsymbol{0}$ and $\bSig = \boldsymbol{I}_{\Da}$\\
    \item[-] $\nu = \nua + \Da - 1$ and $\bPsi = 2\nua\diag(1/a_1,\dots,1/a_{\Da})$\\
    \item[-] $\alpha_d = \dfrac{1}{\mathcal{A}_d^2}$ and $\beta_d = \dfrac{1}{2}$
\end{itemize} 
and the Jacobians are:\\
\begin{itemize}
    \item $\left|J_{\bSigalph\rightarrow \vech(\bCstar)}\right| = 2^{\Da}\prod\limits_{d=1}^{\Da}C_{d,d}^{\Da - d + 2},$ with $C_{d,d}$ is an element in posision $(d,d)$ of matrix $\bC$\\
    \item $\left|J_{a_{1:\Da}\rightarrow \log a_{1:\Da}} \right| =\det \left( \diag(a_1,\dots,a_{\Da})\right) = a_1\times\dots\times a_{\Da}$
\end{itemize}
$\nabla_{\balph_j} \logpriortilde = \nabla_{\balph_j} \log N(\balph_j|\bmualph,\bSigalph) =-\bSigalphinv(\balph_j-\bmualph) $\\

\begin{flalign*}
    \nabla_{\bmualph} \logpriortilde  = &\sum\limits_{j=1}^J \nabla_{\bmualph} \log N(\balph_j|\bmualph,\bSigalph) + \nabla_{\bmualph} \log N(\bmualph|\bmu,\bSig)\\
    = &\sum\limits_{j=1}^J\bSigalphinv(\balph_j-\bmualph) - \bSig^{-1}(\bmualph-\bmu) 
\end{flalign*}

\begin{align*}
&\nabla_{\vech(\bCstar)} \logpriortilde  = \dfrac{\partial}{\partial \vech(\bCstar)} \left[ \sum\limits_{j=1}^J\log N(\balph_j|\bmualph,\bSigalph) + \log \textrm{IW}(\bSigalph|\nu,\bPsi) + \log \left|J_{\bSigalph\rightarrow \vech(\bCstar)}\right|  \right]\\
=&-\dfrac{J+\nu+p+1}{2}\dfrac{\partial}{\partial \vech(\bCstar)} \log |\bSigalph|-\dfrac{1}{2}\dfrac{\partial}{\partial \vech(\bCstar)}\sum\limits_{j=1}^J(\balph_j-\bmualph)^T\bSigalphinv(\balph_j-\bmualph)-\cdots\\
& - \dfrac{1}{2} \dfrac{\partial}{\partial\vech(\bCstar)}\textrm{trace}(\boldsymbol{\Psi}\bSigalphinv) +\dfrac{\partial}{\partial \vech(\bCstar)}\log \left(2^{\Da}\prod\limits_{d=1}^{\Da}C_{d,d}^{\Da - d + 2} \right) \\
=&-(J+\nu+p+1)\vech(\boldsymbol{I}_{\Da}) - \dfrac{1}{2}\vech(\boldsymbol{\overline{C}}) - \dfrac{1}{2}\vech(\boldsymbol{\overline{\overline{C}}}) + \vech\left(\diag(\Da+1,\dots,2) \right)
\end{align*}
where $\boldsymbol{\overline{C}}$ and $\boldsymbol{\overline{\overline{C}}}$ are matrices with the elements are given as followed\\
\begin{center}
    $(\boldsymbol{\overline{C}})_{ij} = \left\{ \begin{array}{lr} 
\boldsymbol{M}_{ij}& \textrm{ if } i\neq j\\
\boldsymbol{M}_{ii}\times (\bC)_{ii} &\textrm{ if } i=j\end{array} \right.$ and  $(\boldsymbol{\overline{\overline{C}}})_{ij} = \left\{ \begin{array}{lr} 
\boldsymbol{H}_{ij}& \textrm{ if } i\neq j\\
\boldsymbol{H}_{ii}\times (\bC)_{ii} &\textrm{ if } i=j\end{array} \right.$\\
\end{center}

$\boldsymbol{M} = -2\bC^{-T}\bC^{-1}\boldsymbol{\Psi}\bC^{-T}$  
and
$\boldsymbol{H} = -2\bC^{-T}\bC^{-1}\sum\limits_{j=1}^J(\balph_j-\bmu)(\balph_j-\bmu)^T\bC^{-T}$ 

The  notation $(\boldsymbol{\overline{C}})_{ij}$ and $(\boldsymbol{\overline{\overline{C}}})_{ij}$ denote the element in row $i$ and column $j$ of matrix  $\boldsymbol{\overline{C}}$ and $\boldsymbol{\overline{\overline{C}}}$, respectively\\

\begin{align*}
    &\nabla_{\log a_d}\logpriortilde = \dfrac{\partial}{\partial\log a_d} \bigg[ \log \textrm{IW}(\bSigalph|\nu,\bPsi) + \log \textrm{IG}(a_d|\alpha_d,\beta_d) + \log\left|J_{a_{1:\Da}\rightarrow \log a_{1:\Da}} \right| \bigg]\\
    &= \dfrac{\partial}{\partial\log a_d} \bigg[ \dfrac{\nu}{2}\log\det\left(2\nua\diag(\dfrac{1}{a_1},\dots,\dfrac{1}{a_{\Da}})
    \right) -\dfrac{1}{2}\tr\left( 2\nua\diag(\dfrac{1}{a_1},\dots,\dfrac{1}{a_{\Da}})\bSigalphinv \right) -\cdots\\ &-(\alpha_d+1)\log a_d -\dfrac{\beta_d}{a_d} + \log a_d \bigg]\\
    &=-\dfrac{\nu}{2} - \dfrac{1}{\mathcal{A}^2_d} + \dfrac{1}{2a_d} +\nu_{\alpha}\dfrac{(\bSigalphinv)_{dd}}{a_d}, \textrm{ for } d=1,\dots,D_{\alpha}
\end{align*}

%\subsection{Compute the gradients}
\subsection*{$\nabla_{\btheta_1} \log p(\by|\btheta_1,\btheta_2)$}
We have
$$ \nabla_{\btheta_1} \log p(\by|\btheta_1,\btheta_2) = \nabla_{\btheta_1}\bigg[ \sum\limits_{j=1}^J\log \textrm{LBA}(\by_j|\balph_j) \bigg] $$
Obviously, $\dfrac{\partial}{\partial \bmualph} \log p(\by|\btheta_1,\btheta_2) = \boldsymbol{0},\quad \dfrac{\partial}{\partial \log a_{1:\Da}} \log p(\by|\btheta_1,\btheta_2) = \boldsymbol{0}$ and $\dfrac{\partial}{\partial \balph_j} \log p(\by|\btheta_1,\btheta_2)$ are given in the appendix of the paper.
\subsection*{$\nabla_{\btheta_1} \log p(\btheta_1,\btheta_2)$}
We have

$$p(\btheta_1,\bSigalph) = \prod\limits_{j=1}^J N(\balph_j|\bmualph,\bSigalph)N(\bmualph|\boldsymbol{0},\boldsymbol{I})\textrm{IW}(\bSigalph|\nu,\bPsi) \prod\limits_{d=1}^{\Da}\textrm{IG}(a_d|\alpha_d,\beta_d)\left| J_{a_d\rightarrow\log a_d}\right|$$
\begin{align*}
\hspace*{-1cm}	\log p(\btheta_1,\bSigalph) &= \sum\limits_{j=1}^J \log N(\balph_j|\bmualph,\bSigalph)+ \log N(\bmualph|\boldsymbol{0},\boldsymbol{I})+ \log\textrm{IW}(\bSigalph|\nu,\bPsi) + \sum\limits_{d=1}^{\Da} \log \textrm{IG}(a_d|\alpha_d,\beta_d) + \log a_d\\
	&\propto -\dfrac{1}{2}\sum\limits_{j=1}^J(\balph_j-\bmualph)^T\bSigalphinv(\balph_j-\bmualph) - \dfrac{1}{2}\bmualph\bmualph^T +\dfrac{\nu}{2}\logdet(\bPsi)-\dfrac{1}{2}\tr (\bPsi\bSigalphinv) +\\
	&+\sum\limits_{d=1}^{\Da}\left\{-(\alpha_d+1)\log a_d - \dfrac{\beta_d}{a_d} + \log a_d\right\}
\end{align*}
It is straight forward to derive
\begin{enumerate}
	\item $\dfrac{\partial}{\partial \balph_j}\log p(\btheta_1,\bSigalph) = -\bSigalphinv(\balph_j-\bmualph)$\\
	\item $\dfrac{\partial}{\partial \bmualph}\log p(\btheta_1,\bSigalph) = \sum\limits_{j=1}^J\bSigalphinv(\balph_j-\bmualph) - \bmualph $\\
	\item $\dfrac{\partial}{\partial \log a_d}\log p(\btheta_1,\bSigalph) = -\dfrac{\nu}{2} - \alpha_d + \dfrac{\beta_d}{a_d} +\nu_{\alpha}\dfrac{(\bSigalphinv)_{dd}}{a_d}$
\end{enumerate}

\subsection*{$\nabla_{\btheta_1}\log q_{\blamb}(\btheta_1)$}
Note that $q_{\blamb}(\btheta_1) = N(\btheta_1|\bmu_{\blamb},BB^T+D^2)$, then $\nabla_{\btheta_1}\log q_{\blamb}(\btheta_1) = -(BB^T+D^2)^{-1}(\btheta_1-\bmu_{\blamb})$
\subsection*{$\nabla_{\btheta_1}\log p(\btheta_2|\btheta_1,\by)$}
$$\log p(\btheta_2|\btheta_1,\by) = \log\textrm{IW}(\bSigalph|\nu,\bPsi') \propto \dfrac{\nu}{2}\logdet(\bPsi') -\dfrac{1}{2}\tr(\bPsi'\bSigalphinv),  $$

with $\bPsi' = 2v_{\alpha}\diag\left( \dfrac{1}{a_1},\dots,\dfrac{1}{a_{\Da}}\right) + \sum\limits_{j=1}^J (\balph_j - \bmualph)(\balph_j - \bmualph)^T$.\\

We have
\begin{enumerate}
	\item $\dfrac{\partial}{\partial \balph_j}\log p(\btheta_2|\btheta_1,\by) = \big( \nu \bPsi'^{-1} - \bSigalphinv\big) (\balph_j-\bmualph)$
	\item $\dfrac{\partial}{\partial \bmualph}\log p(\btheta_2|\btheta_1,\by) = \big( -\nu \bPsi'^{-1} + \bSigalphinv\big)\sum\limits_{j=1}^J (\balph_j-\bmualph)$\\
	\item $\dfrac{\partial}{\partial \log a_d}\log p(\btheta_2|\btheta_1,\by) =-\nu_{\alpha} \dfrac{\nu(\bPsi'^{-1})_{d,d} - (\bSigalphinv)_{d,d}}{a_d} $\\
\end{enumerate}
\begin{figure}[H]
	\hspace*{-2cm}\includegraphics[scale = 0.3]{cov1.jpg}\\
	\hspace*{-2cm}\includegraphics[scale = 0.3]{cov2.jpg}\\
	\caption{The marginal densities of $\bCstar$. Different colors represent four different approximations: blue (VAFC), green (GVA), purple (GCVA), black (CSGVA) and red (PMwG)}
	\label{fig: cov1}
\end{figure}
\begin{figure}[H]
	\hspace*{-2cm}\includegraphics[scale = 0.3]{cov3.jpg}\\
	\vspace*{-3cm}
	\caption{The marginal densities of $\bCstar$. Different colors represent four different approximations: blue (VAFC), green (GVA), purple (GCVA), black (CSGVA) and red (PMwG) (continued)}
	
	\label{fig: cov2}
\end{figure}
